# Supplementary material for: Ultrafast photocurrents in MoSe$_2$ probed by terahertz spectroscopy
Source: arXiv:2008.12203 source file (2020-12-21)
Supplement: Supplementary file 1 [file Supplementary_Ultrafast_photocurrents_in_MoSe2_probed_by_terahertz_spectroscopy.pdf]

# SUPPLEMENTARY INFORMATION

## Ultrafast photocurrents in $MoSe_2$ probed by terahertz spectroscopy

Denis Yagodkin, Lukas Nadvornik, Cornelius Gahl, Tobias Kampfrath, and Kirill I. Bolotin

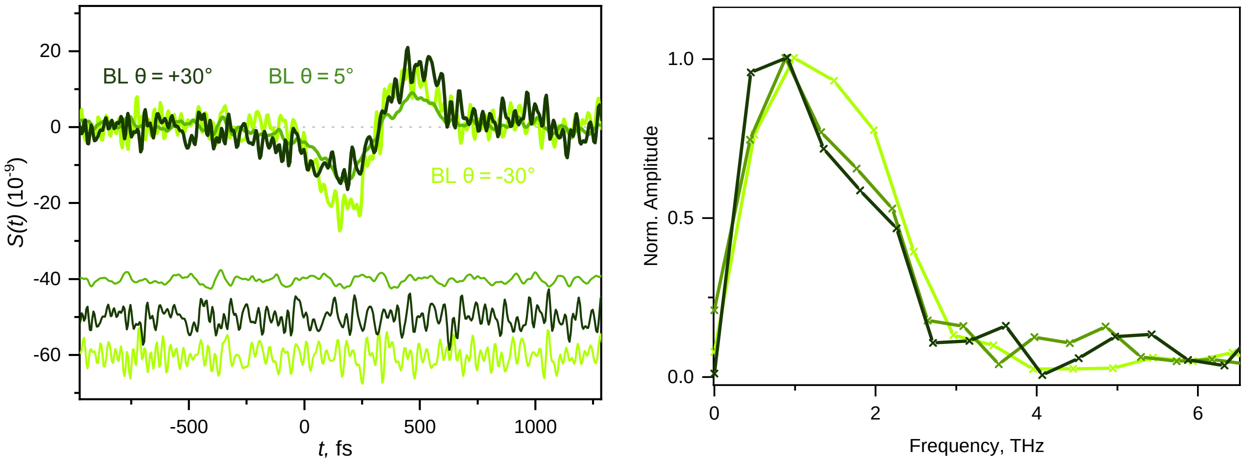


**Fig. S1: Low-frequency emission from the BL $MoSe_2$. Left panel:** Time-dependent THz electric field emitted from the bilayer $MoSe_2$ and measured with the "low-frequency" detector at tilt angles $\theta = +30°; +5°; -30°$ is shown in thick lines shades of green. Thin lines were obtained for corresponding curves by FFT high-pass filter with $\omega_{cut-off} = 3$ THz. Signal above 3 THz is below noise for LF detector. Acquisition time at $\theta = +5°$ is order of magnitude longer which resulted in lower noise. **Right panel:** Fourier transform of the data shown as thick lines in the left panel.

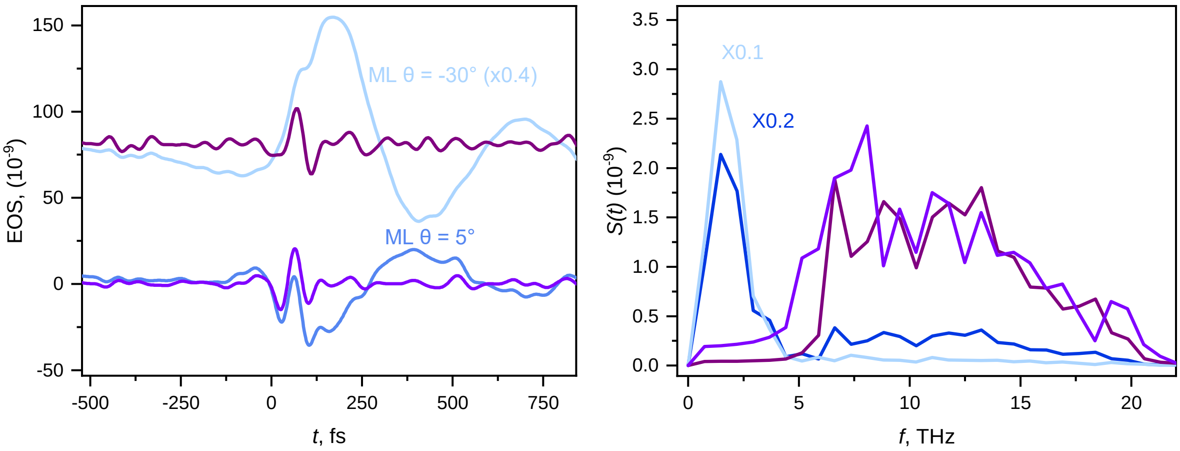


**Fig. S2: High frequency component in ML $MoSe_2$ emission. Left panel:** Time-dependent THz electric field emitted from multilayer $MoSe_2$ and measured with the "low-frequency" detector at tilt angles $\theta = +5°; -30°$ (blue and light blue). The purple and the violet curves were obtained from corresponding signals by filtering with high pass filter $\omega_{cut-off} = 5$ THz in order to highlight HF component of the emission. Note, the violet and the purple curve are not scaled. The initial and the filtered EOS signals for $\theta = -30°$ are offset for clarity. **Right panel:** Fourier transform of the data shown in the left panel. The high-frequency part of the emission has broad distribution centered at around 12 THz.

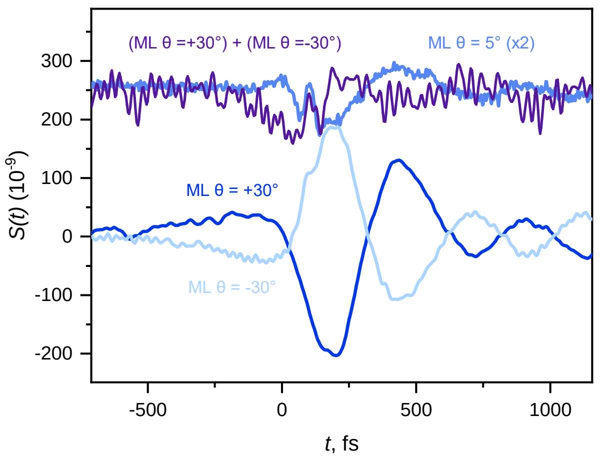


**Fig. S3: Symmetry of the sharp feature in emission at large tilt angles $\theta$.** Time-dependent THz electric field emitted from the multilayer $MoSe_2$ and measured with the "low-frequency" detector at tilt angles $\theta = +30; +5; -30$ is shown in shades of blue (same as, Fig. 2 of the main text). The purple curve is obtained via summation of signals at $\theta = +30°$ and $\theta = -30°$ normalized to mean of peak-to-peak amplitude to account for imperfect setting of tilt angle ($\pm 2°$). Note that the peak seen near zero-delay in the purple curve has near twice the amplitude of the signal at $\theta = -5°$ (note scale factor of 2 for $\theta = -5°$). Indeed, the amplitude of the EOS signal generated by in-plane process is expected to be equal for $\theta = \pm 30°$ (proportional to $cos\,(\theta)$), thus doubles when summed. In contrast, out-of-plane processes are expected to have the opposite amplitudes at $\theta = -30°$ and $+30°$ is (proportional to $\sin(\theta)$). Therefore, sum of out-of-plane processes contributing to signals at $\theta = -30°$ and $+30°$ is zero. Unlike main text where we plot average over multiple scans emission from ML at $\theta = -30°$ and $+30°$, here we use one scan for each angle.

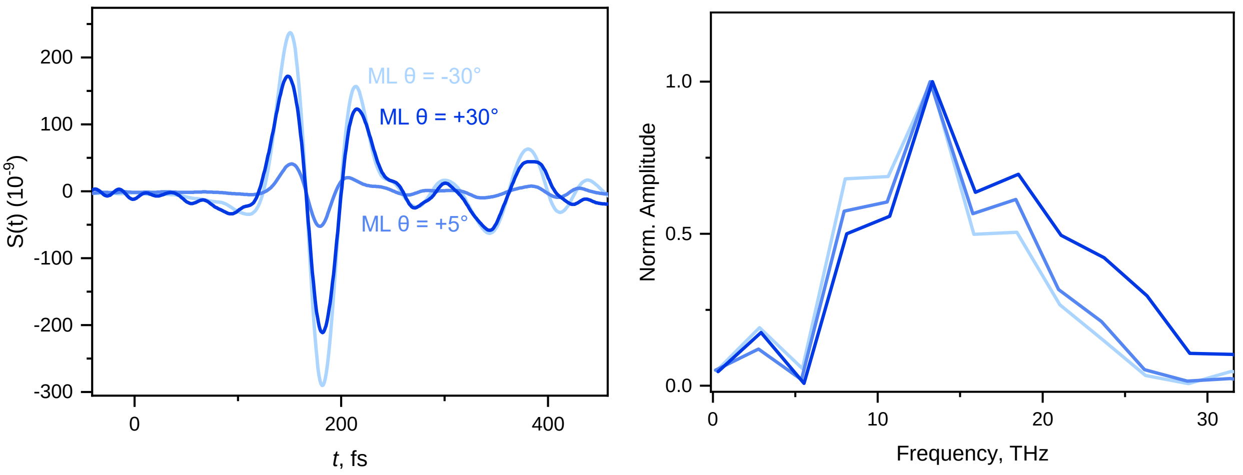


**Fig. S4: High-frequency emission from the multilayer sample. Left panel:** time-dependent THz electric field emitted from multilayer $MoSe_2$ and measured with the "high-frequency" detector at tilt angles $\theta = +30; +5; -30$. **Right panel:** Fourier transform of the data shown in the left panel. The HF emission from the multilayer has the same sign for all tilt angles $\theta$. Such behavior is incompatible with out-of-plane generation for which the sign flip is required due to mirror symmetry with respect to plane orthogonal to the sample ($\theta = 0°$). Therefore, we suggest that the HF emission from the multilayer is of in-plane origin and has complex dependence on $\theta$.

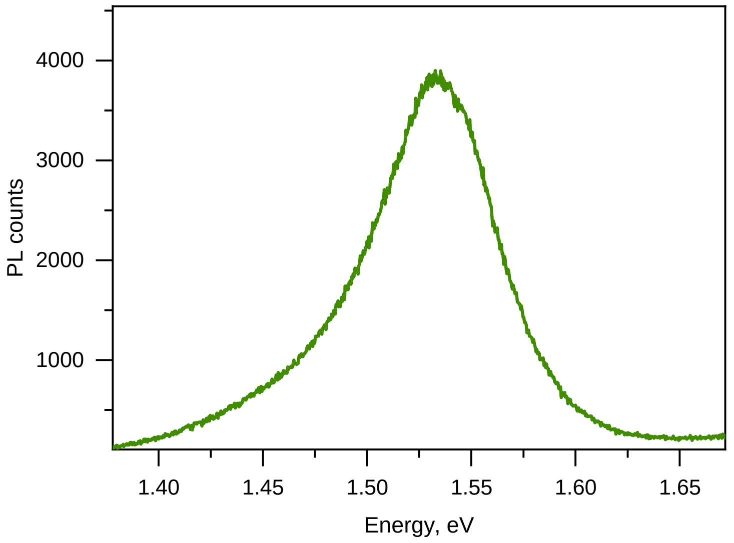


**Fig. S5: Photoluminescence spectrum of the bilayer $MoSe_2$ sample.** The photoluminescence spectrum of the BL sample excited with green laser (532 nm, ~15 μW) at room temperature. The spectrum features excitonic peak centered at ~1.53 eV (810 nm) which overlaps well with pump laser spectrum 1.51 – 1.70 eV (730 - 821 nm).

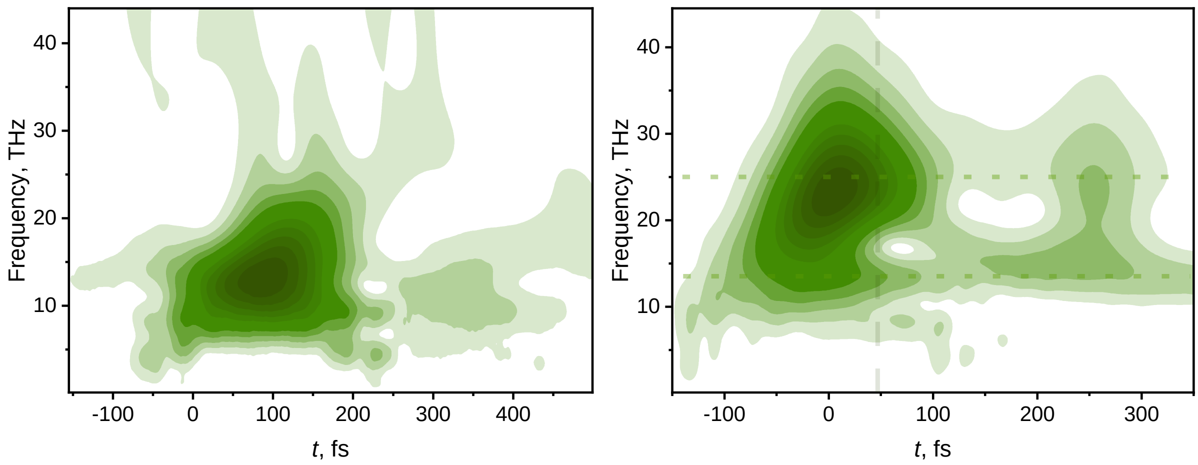


**Fig. S6 Wavelet analysis of HF emission from the BL.** Normalized time-frequency plots of high frequency emission from the BL $MoSe_2$ at tilt angles $\theta = -30^\circ$ (left panel) and $\theta = +5^\circ$ (right panel). The darker is green the more intense. Horizontal doted lines in right panel indicate position of the resonant shift current and the quantum beats peaks. The vertical dashed line shows the center of the Fourier transform window used for Fig. 3b. Wavelet analysis provides both spectral and temporal information of the signal, but at cost of either lower temporal or lower spectral resolution. Fourier transform window of 240 fs is dictated by total duration of the signal, expanding of the window increases influence of parasitic effects such as reflections of the probe/pump and absorption and reemission on water vapor. The first and the last point of the window is chosen such the difference of the signal at these points is close to zero, to minimize influence of the edges to Fourier transform.

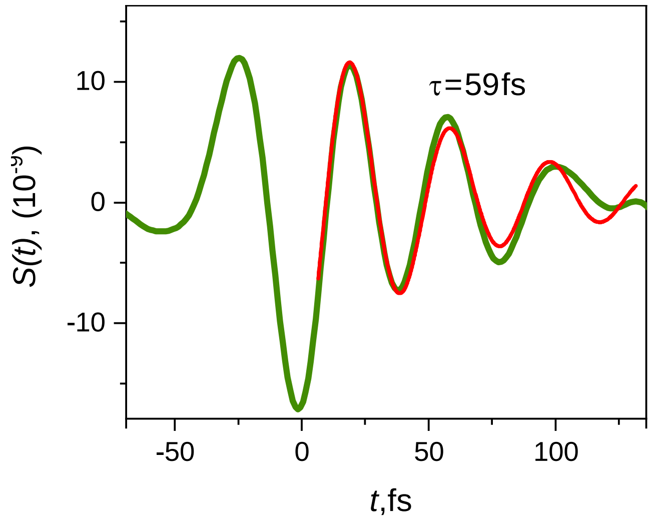


**Fig. S7: Decay time of oscillations in the HF emission from the BL.** The HF frequency emission from the BL $MoSe_2$ at $\theta = +5°$ (green), copying Fig. 3a of the main text. The red curve is fit to $A \cdot e^{-t/\tau} sin(t)$, which yields decay constant $\tau = 59$ fs.

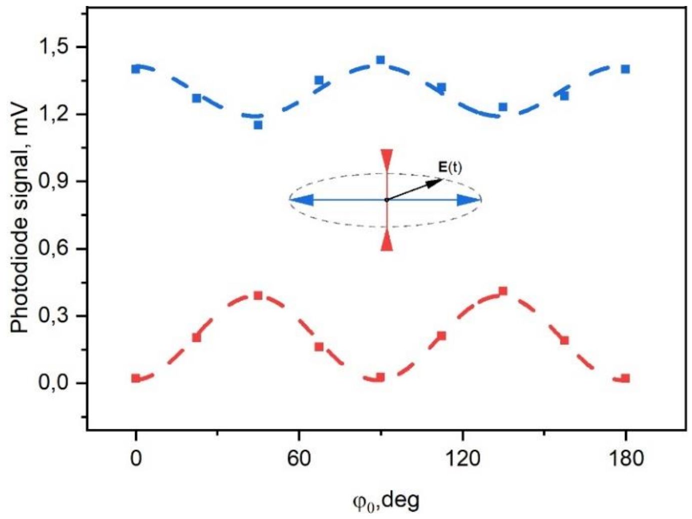


**Fig. S8:** The dependency of the pump power at the sample position for major (blue) and minor (red) axes of elliptical polarization on angle $\varphi_0$ (squares) equal to the doubled angle of $\lambda/2$ - plate measured at the sample surface. Dashed curves – fit to $sin^2\, \varphi_0$. Inset: Major and minor axis of the elliptically polarized light.

# Supplementary note 1

The electro-optical signal $S(t)$ provides sufficient information about the emitted field, but the properties of the sampling crystal or measurement setup affect the readings. Below, we discuss how to avoid setup or detection crystal related effects by directly reconstructing the emitted field.

We used a reference emitter, namely spintronic THz emitter (STE) [1], to extract the current from the EOS signal $S(t)$. The STE was calibrated to ZnTe emitter with the theoretically calculated emission spectrum [2]. The detected signal can be found via

$$S(t) = (h * E)(t)$$

where $S(t)$ is the measured EOS signal, $h(t)$ is the response function of the setup (includes the propagation of THz radiation to the detector and the detector response), and $E(t)$ is emitted THz field, $*$ the symbol represents convolution. This equation then can be solved to extract the electric field. We extract h(t) from calibration measurements where the $E(t)$ is theoretically calculated emission of STE and $S(t)$ is EOS signal. Then we use extracted $h(t)$ and measured emission from the sample $S(t)$ to reconstruct $E(t)$. The simplest way of solving is to take a Fourier transformation of both parts of the equation. Then convolution becomes multiplication of the spectral functions. Next, the electric field near the sample can be found by dividing the Fourier transform of measured emission by Fourier transform of the response function $E(\omega) = S(\omega)/h(\omega)$.

# Supplementary note 2

In this supplementary note, we derive a fitting function for the dependence of the EOS signal on the polarisation of the pump pulse in near-orthogonal geometry $\theta = 5°$.

The nonlinear response of media is described by polarization. The nonlinear contribution to it under optical excitation reads [1]:

$$P^{a}_{\text{rect}}(t) = 2\chi_{2}{}^{abc}_{\text{rect}}(\omega_0)E^{b}_{\text{env}}(t)E^{c}_{\text{env}}(t)$$

where $P^{a}_{\text{rect}}(t)$ is $a$ component of polarization vector, $\chi_{2}{}^{abc}_{\text{rect}}(\omega_0)$ is $abc$ component of susceptibility tensor, $E^{b}_{\text{env}}(t); E^{c}_{\text{env}}(t)$ are $b$ and $c$ components of the envelope of electrical field vector, $\omega_0$ is the frequency of the carrier wave. The polarization vector can be converted to current via $j(t) = \frac{\partial P(t)}{\partial t}$ or in frequnecy domain $j(\omega) = i\omega P(\omega)$. Combining it, the current density vector $j^{\mu}$ as a function of second-order susceptibility tensor $\sigma^{\mu'}_{\lambda'\nu'}$ and electric field $E^{\mu}$ [1]:

$$j^{\mu'} = \sigma^{\mu'}_{\lambda'\nu'}(E^{\lambda'}E^{\nu'}) = \sigma^{\mu'}_{(\lambda'\nu')}\Sigma^{(\lambda'\nu')}, \tag{1}$$

where $\Sigma^{(\lambda'\nu')}$ is contracted using joint indexes (Voigt notation) $\lambda'\nu'$ form of $(E^{\lambda'}E^{\nu'})$. Since the optical pump is non-monochromatic, this contraction is possible when the system has Kleinmann symmetry. Which is formulated as permutational invariance of the susceptibility withouth permuting frequency $\chi_2{}^{abc}(\omega_0 = \omega_1 + \omega_2; \omega_1; \omega_2) = \cdots = \chi_2{}^{bca}(\omega_0 = \omega_1 + \omega_2; \omega_1; \omega_2) = \chi_2{}^{cba}(\omega_0 = \omega_1 + \omega_2; \omega_1; \omega_2)$. It is shown that this symmetry holds when the medium is transparent for excitation [2]. Although the laser we used is in resonance with the excitonic transition in our material, Kleinmann symmetry is still present in the medium due to the high symmetry of $MoSe_2$. Monolayer $MoSe_2$ has symmetry $\bar{6}\text{m}2$ ($\text{D}_{3\text{h}}$) for this symmetry second-order tensor has one independent component and is originally symmetric for permutations: $\chi_{xxx} = -\chi_{xxy} = -\chi_{xyx} = -\chi_{yxx}$ [3]. Therefore, the Kleinman symmetry holds and Voigt notation is justified.

Voigt notation reduces 3D tensor into 2D matrix which is simpler to work with, but the basis becomes more complex. The second-order susceptibility tensor has three indexes and can be

expressed as 3D array, where two indexes run overall coordinates of each field vector and one index corresponds to $x; y; z$ components of the current. On the other hand, when two electric field indexes are joint we have one index for current running over $\{e_1; e_2; e_3\}$ and another one going over $\{e_1 \otimes e_1; e_2 \otimes e_2; e_3 \otimes e_3; \frac{(e_2 \otimes e_3 + e_3 \otimes e_2)}{\sqrt{2}}; \frac{(e_1 \otimes e_3 + e_3 \otimes e_1)}{\sqrt{2}}; \frac{(e_1 \otimes e_2 + e_2 \otimes e_1)}{\sqrt{2}}\}$, where the denominator $\sqrt{2}$ is used to preserve orthonormality.

In simple $\{e_1; e_2; e_3\}$ - basis a vector, say, current is rotated via rotation matrix $R_{\mu}^{\mu'}$:

$$j^{\mu'} = R_{\mu}^{\mu'} j^{\mu} \quad (2)$$

To have a rotation matrix $R_{\lambda\nu}^{\lambda'\nu'}$ in the joint indexes basis would be ideal for rotation of any matrix and second-order susceptibility in particular. Such rotation matrix should transform coordinates of $\Sigma^{\lambda\nu}$as well:

$$j^{\mu'} = \sigma_{\lambda'\nu'}^{\mu'} \Sigma^{\lambda'\nu'} = \sigma_{\lambda'\nu'}^{\mu'} R_{\lambda\nu}^{\lambda'\nu'} \Sigma^{\lambda\nu} \quad (3)$$

Combining eq. 2 and eq. 3 we obtain

$$j^{\mu} = R_{\mu'}^{\mu} \sigma_{\lambda'\nu'}^{\mu'} R_{\lambda\nu}^{\lambda'\nu'} \Sigma^{\lambda\nu} \quad (4)$$

Then

$$\sigma_{\lambda\nu}^{\mu} = R_{\mu'}^{\mu} \sigma_{\lambda'\nu'}^{\mu'} R_{\lambda\nu}^{\lambda'\nu'} \quad (5)$$

where $R_{\mu'}^{\mu}$ is inverse to $R_{\mu}^{\mu'}$ rotation matrix. In order to find $R_{\lambda\nu}^{\lambda'\nu'}$ we derive a representation of the rotated basis in the initial one. This yields:

$$R_{\lambda\nu}^{\lambda'\nu'} = \begin{pmatrix} R_{11}^2 & R_{12}^2 & R_{13}^2 & \sqrt{2}R_{12}R_{13} & \sqrt{2}R_{11}R_{13} & \sqrt{2}R_{11}R_{12} \\ R_{21}^2 & R_{22}^2 & R_{23}^2 & \sqrt{2}R_{22}R_{23} & \sqrt{2}R_{21}R_{23} & \sqrt{2}R_{22}R_{21} \\ R_{31}^2 & R_{32}^2 & R_{33}^2 & \sqrt{2}R_{33}R_{32} & \sqrt{2}R_{33}P_{31} & \sqrt{2}R_{31}R_{32} \\ \sqrt{2}R_{21}R_{31} & \sqrt{2}R_{22}R_{32} & \sqrt{2}R_{23}R_{33} & (R_{22}R_{33} + R_{23}R_{32}) & (R_{21}R_{33} + R_{31}R_{23}) & (R_{21}R_{32} + R_{31}R_{22}) \\ \sqrt{2}R_{11}R_{31} & \sqrt{2}R_{12}R_{32} & \sqrt{2}R_{13}R_{33} & (R_{12}R_{33} + R_{32}R_{13}) & (R_{11}R_{33} + R_{13}R_{31}) & (R_{11}R_{32} + R_{31}R_{12}) \\ \sqrt{2}R_{11}R_{21} & \sqrt{2}R_{22}R_{12} & \sqrt{2}R_{13}R_{23} & (R_{12}R_{23} + R_{22}R_{13}) & (R_{11}R_{23} + R_{21}R_{13}) & (R_{11}R_{22} + R_{21}R_{12}) \end{pmatrix}$$

where each term $R_{ij}$ is the corresponding component of the 2D rotational matrix.

We test this approach with several examples before utilizing complex $R_{\lambda\nu}^{\lambda'\nu'}$ - "6D" rotation matrix for rotation of the susceptibility tensor. Starting from field vector $E_{\nu} = (1,1,0)$ we derive $\Sigma_{\nu\mu}$ which we than rotate by $-45°$ with help of the matrix above. This results in $\Sigma_{\nu\mu} = (2\ 0\ 0\ 0\ 0\ )$. We also tested a more complex case where $E_{\nu} = \left(\frac{\sqrt{3}}{2}, \frac{\sqrt{2}}{2}, 0\right)$ we rotate it by $-60°$ and get $\Sigma_{\nu\mu} = (1\ 0\ 0\ 0\ 0\ )$. Both results coincide with obtained by first rotation of $E_{\nu}$ and then deriving $\Sigma_{\nu\mu}$.

Now, we apply the rotation approach to the TMDCs. Monolayer $MoSe_2$ has symmetry $\bar{6}m2$ $(D_{3h})$ which yields the following second-order tensor [4]:

$$\sigma = d \begin{pmatrix} 0 & 0 & 0 & 0 & -\sqrt{2} \\ -1 & 1 & 0 & 0 & 0 \\ 0 & 0 & 0 & 0 & 0 \end{pmatrix}, \quad (6)$$

where due to choice of the basis (divided by $\sqrt{2}$) in the last column we have $-\sqrt{2}$ instead of conventional $-1$. The second-order tensor of that symmetry group has only one coefficient $d$ which we drop in the calculation and will add at the end.

Since the initial angle of the crystal is unknown, we account for this by rotation of $\sigma$ by variable angle $\varphi_0$. We start with 2D rotation matrix and inverse to it:

$$R = \begin{pmatrix} \cos\varphi_0 & -\sin\varphi_0 & 0 \\ \sin\varphi_0 & \cos\varphi_0 & 0 \\ 0 & 0 & 1 \end{pmatrix} \qquad R^{-1} = \begin{pmatrix} \cos\varphi_0 & \sin\varphi_0 & 0 \\ -\sin\varphi_0 & \cos\varphi_0 & 0 \\ 0 & 0 & 1 \end{pmatrix} \tag{7}$$

Next, we derive "6D" rotational matrix from eq. 7

$$R_{\lambda\nu}^{\lambda'\nu'} = \begin{pmatrix} \cos^2\varphi_0 & \sin^2\varphi_0 & 0 & 0 & 0 & -\sqrt{2}\cos\varphi_0\sin\varphi_0 \\ \sin^2\varphi_0 & \cos^2\varphi_0 & 0 & 0 & 0 & \sqrt{2}\sin\varphi_0\cos\varphi_0 \\ 0 & 0 & 1 & 0 & 0 & 0 \\ 0 & 0 & 0 & \cos\varphi_0 & \sin\varphi_0 & 0 \\ 0 & 0 & 0 & -\sin\varphi_0 & \cos\varphi_0 & 0 \\ \sqrt{2}\sin\varphi_0\cos\varphi_0 & -\sqrt{2}\sin\varphi_0\cos\varphi_0 & 0 & 0 & 0 & \cos^2\varphi_0 - \sin^2\varphi_0 \end{pmatrix}$$

First, we multiply the second-order susceptibility tensor (eq. 6) by this "6D" rotational matrix:

$$\sigma R_{\lambda\nu}^{\lambda'\nu'} = \mathrm{d}\begin{pmatrix} -2\sin\varphi_0\cos\varphi_0 & 2\cos\varphi_0\sin\varphi_0 & 0 & 0 & 0 & -\sqrt{2}(\cos^2\varphi_0 - \sin^2\varphi_0) \\ -\cos^2\varphi_0 + \sin^2\varphi_0 & \cos^2\varphi_0 - \sin^2\varphi_0 & 0 & 0 & 0 & \sqrt{2}(2\sin\varphi_0\cos\varphi_0) \\ 0 & 0 & 0 & 0 & 0 & 0 \end{pmatrix} =$$

$$= \mathrm{d}\begin{pmatrix} -\sin2\varphi_0 & \sin2\varphi_0 & 0 & 0 & 0 & -\sqrt{2}\cos2\varphi_0 \\ -\cos2\varphi_0 & \cos2\varphi_0 & 0 & 0 & 0 & \sqrt{2}\sin2\varphi_0 \\ 0 & 0 & 0 & 0 & 0 & 0 \end{pmatrix} \tag{9}$$

In accordance with eq. 5 we should multiply the result by the $R^{-1}$ (eq. 7) from the left-hand side

$$R^{-1}\sigma R = \mathrm{d}\begin{pmatrix} -\sin3\varphi_0 & \sin3\varphi_0 & 0 & 0 & 0 & -\sqrt{2}\cos3\varphi_0 \\ -\cos3\varphi_0 & \cos3\varphi_0 & 0 & 0 & 0 & \sqrt{2}\sin3\varphi_0 \\ 0 & 0 & 0 & 0 & 0 & 0 \end{pmatrix} \tag{10}$$

In the experiment, the polarisation state of the optical pulse is perturbed by hemispherical mirrors. To account for this effect, we assume that the initial linear polarization becomes elliptical as perturbed and then the elliptically polarized light is rotated via $\lambda/2$ plate. Then the "6D" electric field vector $\Sigma_{\nu\mu}$ is

$$\begin{pmatrix} E_a^2 \\ E_b^2 \\ 0 \\ 0 \\ 0 \\ 0 \\ \sqrt{2}E_aE_b \end{pmatrix} \equiv \begin{pmatrix} a^2 \\ b^2 \\ 0 \\ 0 \\ 0 \\ 0 \\ \sqrt{2}ab \end{pmatrix} \tag{11}$$

where $E_a; E_b$ are the strength of the electric field along major and minor axis respectively. The phase is irrelevant since considered SOEs are insensitive to it [1]. The effect of $\lambda/2$ - plate is described by "6D" rotation matrix with $\varphi$ — doubled angle of the $\lambda/2$ - plate.

$$R_{\lambda\nu}^{\lambda'\nu'}\Sigma_{\lambda'\nu'} = \begin{pmatrix} a^2\cos^2\varphi + b^2\sin^2\varphi - 2ab\sin\varphi\cos\varphi \\ a^2\sin^2\varphi + b^2\cos^2\varphi + 2ab\cos\varphi\sin\varphi \\ 0 \\ 0 \\ 0 \\ \sqrt{2}\sin\varphi\cos\varphi(a^2 - b^2) + \sqrt{2}ab(\cos^2\varphi - \sin^2\varphi) \end{pmatrix} \tag{12}$$

Finally, we combine results eq. 12 and eq. 10 in $j^{\mu'} = \sigma^{\mu'}_{\lambda'\nu'}\Sigma^{\lambda'\nu'}$ and obtain

$$j^{\mu'} = \mathrm{d}\begin{pmatrix} -\sin3\varphi_0(a^2\cos^2 2\varphi + b^2\sin^2 2\varphi - 2ab\sin\varphi\cos\varphi) + \\ \cos3\varphi_0(a^2\cos^2 2\varphi + b^2\sin^2 2\varphi - 2ab\sin\varphi\cos\varphi) + \\ 0 \\ \\ +\sin3\varphi_0(a^2\sin^2 2\varphi + b^2\cos^2 2\varphi + 2ab\sin\varphi\cos\varphi) - \\ +\cos3\varphi_0(a^2\sin^2 2\varphi + b^2\cos^2 2\varphi + 2ab\cos\varphi\sin\varphi) + \\ 0 \\ \\ -2\cos3\varphi_0[(a^2-b^2)\sin\varphi\cos\varphi + ab(\cos^2 2\varphi - \sin^2 2\varphi)] \\ +2\sin3\varphi_0[(a^2-b^2)\sin\varphi\cos\varphi + ab(\cos^2 2\varphi - \sin^2 2\varphi)] \\ 0 \end{pmatrix} \tag{13}$$

Since we use p-polarized optical detection, we are sensitive only to $x$-component of the current:

$$\begin{aligned} j_x/\mathrm{d} &= -\sin3\varphi_0(a^2\cos^2 2\varphi + b^2\sin^2 2\varphi - 2ab\sin\varphi\cos\varphi) + \\ &+ \sin3\varphi_0(a^2\sin^2 2\varphi + b^2\cos^2 2\varphi + 2ab\sin\varphi\cos\varphi) - \\ &- 2\cos3\varphi_0[(a^2-b^2)\sin\varphi\cos\varphi + ab(\cos^2 2\varphi - \sin^2 2\varphi)] \\ &= [(\mathrm{b}^2 - \mathrm{a}^2)\sin(2\varphi + 3\varphi_0) - 2\mathrm{ab}\cos(2\varphi + 3\varphi_0)] \end{aligned} \tag{14}$$

Next, we include the second layer of $MoSe_2$ in the model. Current that each layer produces flows in opposite directions since one flake is rotated by 180° with respect to another. Therefore, the initial rotation angle $\varphi_{0;2^{nd}}$ second flake is equal to $\varphi_{0;1^{st}} + \pi$, which infers $\sin\left(2\varphi + 3\varphi_{0;2^{\mathrm{nd}}}\right) = -\sin(2\varphi + 3\varphi_0) \equiv -\sin\left(2\varphi + 3\varphi_{0;1^{\mathrm{st}}}\right)$. Then the sum of currents in two flakes:

$$j_{tot,x} = j_{1^{\mathrm{st}},x} + j_{2^{\mathrm{nd}},\mathrm{x}} = j_{1^{\mathrm{st}},x} - \alpha j_{1^{\mathrm{st}},x} = (1-\alpha)\, j_{1^{\mathrm{st}},x} \tag{15}$$

where $j_{tot,x}; j_{1^{\mathrm{st}},x}; j_{2^{\mathrm{nd}},x}$ are $x$ components of the total current, currents in the first flake, and the second flake respectively. Paramiter $\alpha$ accounts for braking of symmetry between top and bottom flake due to $MoSe_2$/Air and $MoSe_2$/Sapphire interfaces asymmetry [5]. Finally, we obtain the fitting function

$$j_{tot,x} = j_{other} + A[f(\varphi)\sin(2\varphi + 3\varphi_0) + g(\varphi)\cos(2\varphi + 3\varphi_0)], \tag{16}$$

Here $f(\varphi) = \ b(\varphi)^2 - a(\varphi)^2$ and $g(\varphi) = \ -2a(\varphi)b(\varphi)$, $a(\varphi); b(\varphi)$ are measured dependence of pump polarization on the angle of $\lambda/2$ -waveplate (Fig. S9) , $j_{other}$ is a polarization-independent offset (either experimental offset or an effect of different nature). $A$ is the amplitude of the SOE.

One would expect 3-fold symmetry of the current on angle $\varphi$ of pump polarization when in eq.16 case, it is 2-fold symmetric. Note, the fitting function is 3-fold symmetric with the angle of the crystalline structure $\varphi_0$. For rotation of the sampling beam polarization the current is 3-fold symmetric on $\varphi$ . Indeed, projection of the current eq. 13 on to directionality vector $(\cos\varphi; \sin\varphi; 0)$ representing rotation of the sampling beam (detector) is

$$j = j_{other} + Af(\varphi)\sin[3(\varphi + \varphi_0)] \tag{17}$$

This example illustrate that the obtained eq. 16 is consistent with initially expected dependence for this symmetry.

Above we have derived the THz emission in near-orthogonal geometry. That approximation simplifies the derivation and makes possible direct calculation without numerical methods. Once angle $\theta$ becomes significantly non-zero, we should also include the reflection of an optical pulse from sapphire along with “6D” rotation matrix for $\theta$. The letter is done with the help of Fresnel equation for linear polarization $R_s$ and $R_p$, it reads:

$$R_{\mathrm{s}} = \left| \frac{n_1 \cos\theta_{\mathrm{i}} - n_2 \sqrt{1 - \left(\frac{n_1}{n_2} \sin\theta_{\mathrm{i}}\right)^2}}{n_1 \cos\theta_{\mathrm{i}} + n_2 \sqrt{1 - \left(\frac{n_1}{n_2} \sin\theta_{\mathrm{i}}\right)^2}} \right|^2 \tag{31}$$

$$R_{\mathrm{p}} = \left| \frac{n_1 \sqrt{1 - \left(\frac{n_1}{n_2} \sin\theta_{\mathrm{i}}\right)^2} - n_2 \cos\theta_{\mathrm{i}}}{n_1 \sqrt{1 - \left(\frac{n_1}{n_2} \sin\theta_{\mathrm{i}}\right)^2} + n_2 \cos\theta_{\mathrm{i}}} \right|^2, \tag{32}$$

where $n_1$; $n_2$ are refractive indexes of two media at the interface, $\theta_i$ is the angle of incidence. The refractive index of $MoSe_2$ at $800$ nm is $n_{\mathrm{MoSe_2}} = 5$ [5] and sapphire has refractive index $n_{\mathrm{sapphire}} = 1.76$ [6] at this wavelength. The refractive index of air is assumed to be $1$ in THz and visible ranges of the spectrum. The reflection of the THz radiation at the interfaces $MoSe_2$/air and $MoSe_2$/sapphire is similar and can be derived either from Fresnel equations or boundary conditions of the electromagnetic field. Both approaches lead to the following relation between emitted p-polarized field and current in the sample [7]

$$E_p(\theta, \varphi_0, \varphi) = \frac{2\gamma\left[(\gamma \sin\theta - \sin\theta\cos\theta] j_z(\theta, \varphi_0, \varphi) + \left(\cos\theta\gamma + \sin^2\theta\right) j_x(\theta, \varphi_0, \varphi)\right)}{\gamma + n_{THz}{}^2 \cos\theta},$$

where $\gamma = \sqrt{n_{THz}^2 - \sin^2\theta}$; $n_{THz} = 20$ [8] is the refractive index of $MoSe_2$ at terahertz frequencies, $\theta$ is tilt angle , $\varphi$ is twice the angle of $\lambda/2$-plate, $\varphi_0$ is the initial angle of the $MoSe_2$ about normal to the surface, $j_x$ and $j_z$ are components of the current which are as before equal to $j_\mu(\theta, \varphi_0, \varphi) = \sigma_\mu^{\lambda\nu}(\theta, \varphi_0)\Sigma_{\lambda\nu}(\theta, \varphi)$. Please note that a significant part of the radiation doesn't propagate towards detector due to refractive indexes mismatch. This provides an opportunity for optimization of the THz emission from $MoSe_2$.

# Bibliography

[1] F. Nastos and J. E. Sipe, "Optical rectification and shift currents in GaAs and GaP response: Below and above the band gap," *Physical Review B,* 2006.

[2] P.-F. Brevet, "Kleinmann symmetry," in *Surface Second Harmonic Generation*, PPUR presses polytechniques, 1997, p. 45.

[3] Y.-R. Shen, The Principles of Nonlinear Optics, Wiley, 2003.

[4] M. de Jong, W. Chen, H. Geerlings, M. Asta and K. A. Persson, "A database to enable discovery and design of piezoelectric materials," *Scientific Data,* 2015.

[5] A. R. Beal and H. P. Hughes, "Kramers-Kronig analysis of the reflectivity spectra of 2H-MoS2, 2H-MoSe2and 2H-MoTe2," *Journal of Physics C: Solid State Physics,* 1979.

[6] J. O. Tocho and F. Sanjuan , "Optical properties of silicon, sapphire, silica and glass in the Terahertz range," in *Latin America Optics and Photonics Conference*, OSA, 2012.

[7] J. Shan and T. F. Heinz, "Terahertz radiation from semiconductors," in *Ultrafast Dynamical Processes in Semiconductors*, Springer, 2004, pp. 1-56.

[8] G. Papari, C. Koral, T. Hallam, G. Duesberg and A. Andreone, "Terahertz Spectroscopy of Amorphous WSe2 and MoSe2 Thin Films," *Materials,* 2018.
